# Supplementary material for: Proto-lm: A Prototypical Network-Based Framework for Built-in Interpretability in Large Language Models
Source: arXiv:2311.01732 source file (2023-11-12)
Supplement: Supplementary file 2 [file additional_faith.tex]

Let $\hat{y}_i$ be the prediction of a model $\mathcal{M}$ on $x_i$. let $pr_{\hat{y}_i}$ be the output logit of $M$ for $\hat{y}_i$. Moreover, let $pr_{\hat{y}_i}(P \setminus p^k_i)$ be the output logit when $p^k_i$ prototypes are removed from the prototypical layer and let $pr_{\hat{y}_i}(p^k_i)$ be the output logit when only $p^k_i$ are retained, we calculate Comprehensiveness (Comp) and Sufficiencey (Suff) as follows:
\begin{equation}
    \text{Comp} = \frac{pr_{\hat{y}_i} - pr_{\hat{y}_i}(P \setminus p^k_i) }
                {pr_{\hat{y}_i}}
    \label{eq:comp_eq}
\end{equation}

\begin{equation}
    \text{Suff} = \frac{pr_{\hat{y}_i} - pr_{\hat{y}_i}(p^k_i) }
                {pr_{\hat{y}_i}}
    \label{eq:suff_eq}
\end{equation}

The Comp and Suff reported in Fig \ref{fig:comp_suff} are the mean Comp and Suff over the tasks of SST2, QNLI, MNLI and SST5. Our formulation of prototype Comp and Suff are inspired by \citet{deyoung2019eraser}. We note here again that under this formulation, a \textbf{lower} sufficiency is \textit{better} i.e., a small amount of reduction in model confidence when only salient features are retained.
